# Supplementary material for: Canonical, Stable, General Mapping using Context Schemes
Source: arXiv:1501.04128 source file (2015-06-11)
Supplement: Supplementary file 1 [file supplement.pdf]

BIOINFORMATICS

Vol. 00 no. 00 2015
Pages 1–3

# Supplement: Canonical, Stable, General Mapping using Context Schemes

Novak, Adam M[1], Rosen, Yohei[2], Haussler, David[1], and Paten, Benedict[1]

[1]UC Santa Cruz Genomics Institute, 1156 High Street, Santa Cruz, CA 95064
[2]NYU School of Medicine, 550 First Avenue, New York, NY 10016

Received on XXXXX; revised on XXXXX; accepted on XXXXX

Associate Editor: XXXXXXX

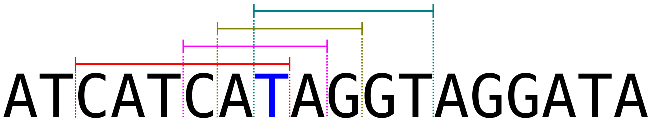


Fig. S1: An example of natural contexts. The blue base "T" is shown together with four of its natural contexts: (CATCA, **T**, ) in red, (CA, **T**, A) in magenta, (A, **T**, AG) in gold, and (, **T**, AGGT) in teal. These contexts are minimal, since none of them can be shortened at either end and still be unique to the position in question. Under the natural context scheme, these contexts would constitute the context set for the blue "T"'s position. Any "T" appearing in one of these contexts, and not in a context assigned to any other base, would be mapped to the blue "T".

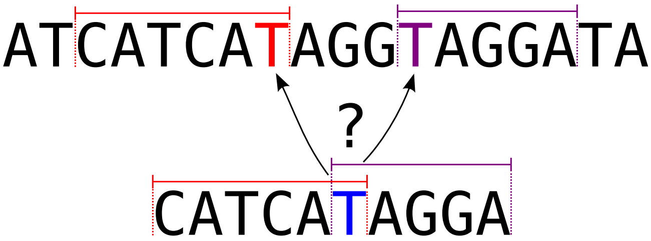


Fig. S2: An example of conflict in the natural mapping scheme, when one base in the query (bottom) matches contexts for multiple positions in the reference (top). One base (blue) in the query occurs in two overlapping query substrings (red and purple), which are the context strings of natural contexts of two different positions (red and purple) in the reference. The "T" being mapped matches both these reference positions. In this case, that "T" must remain unmapped because of the conflict.

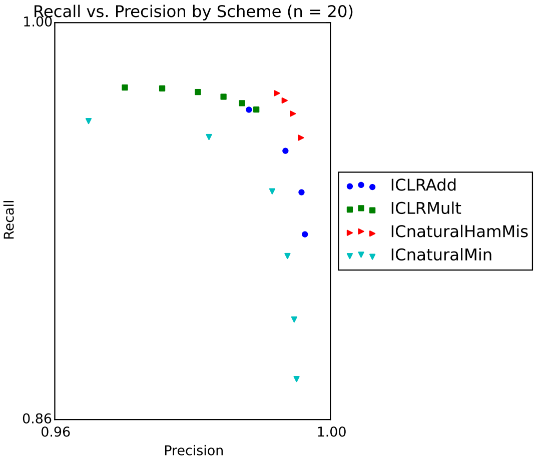


Fig. S3: Comparison between the $\alpha'$-$\beta'$-natural mapping scheme (red rightwards triangles) and a variety of other scheme. Two of the schemes are based on mapping on the left and right sides independently with two different mechanisms for calculating minimum context length (green squares for multiplying the length at which a unique mapping is found, and blue circles for adding to it), while one scheme is the natural scheme with a flat minimum context length (cyan downwards triangles). Parameters for each scheme were varied to produce the precision-recall trade-off curves shown here. Precision and recall were calculated against the GRC alignments with mismatching bases left aligned.

## S1 HEURISTIC ALGORITHM FOR THE $\alpha$-$\beta$-NATURAL CONTEXT-DRIVEN MAPPING SCHEME

Unfortunately, algorithms built on efficient substring indexes to implement the $\alpha$-$\beta$-natural scheme require tracking a number of potential matches that is exponential in both $\alpha$ and $\beta$ parameters. Here, we present an algorithm that heuristically approximates the $\alpha$-$\beta$-natural scheme. As discussed in the main text, the basic idea of the algorithm, inspired by existing seed-and-extend hashtable methods and chaining methods like BWA-MEM, is to chain exact matches separated by mismatching gaps, until a sufficient $\alpha$-separation is obtained (Li and Homer, 2010; Li, 2013).

As defined in the main text, a **minimal unique substring (MUS)** for a reference is a shortest length substring that appears once in the reference. Two MUSes are disjoint if they do not overlap. We define $\alpha'$ as the maximum number of disjoint MUSes within a context string. It is easy to verify that $\alpha'$ is a lower bound on $\alpha$.

© Oxford University Press 2015.

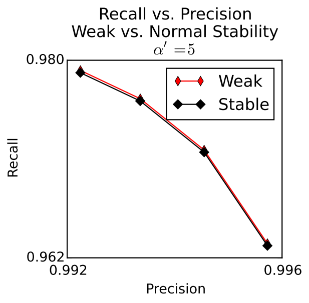


(a)

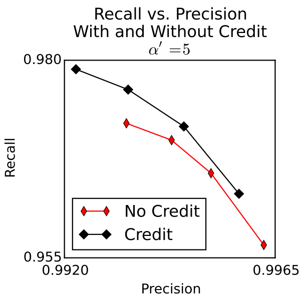


(b)

Fig. S4: Effects of credit and stability parameters on MHC alignment quality. Points shown in S4a and S4b are averages of alt-loci alignments.

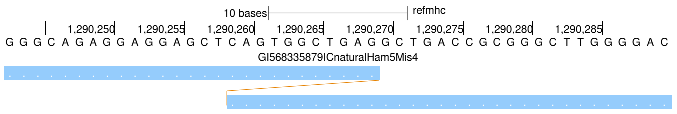


(a)

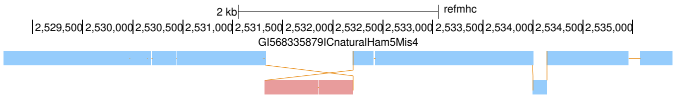


(b)

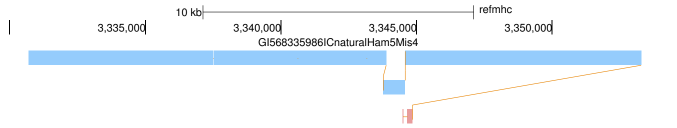


(c)

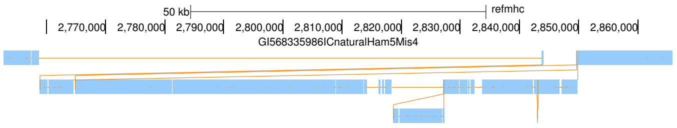


(d)

Fig. S5: A tandem duplication (S5a), inversion (S5b), simple inverting long-range duplication (S5c) and a more complex large-scale rearrangement (S5d) detected by the $\alpha' = 5$, $\beta' = 4$ natural scheme, as rendered by the UCSC Genome Browser (Nguyen *et al.*, 2014).

A query substring $x$ of length $n$ contains at most $n$ MUS instances. The set of MUS instances contained in $x$ can be partitioned by the MUM instance they are part of because a MUS instance must be contained in exactly one MUM instance (although it may overlap several). Using an algorithm similar to that given in the main text for MUMs, a substring index data structure of the strings in a reference can be used to find the set of MUS instances

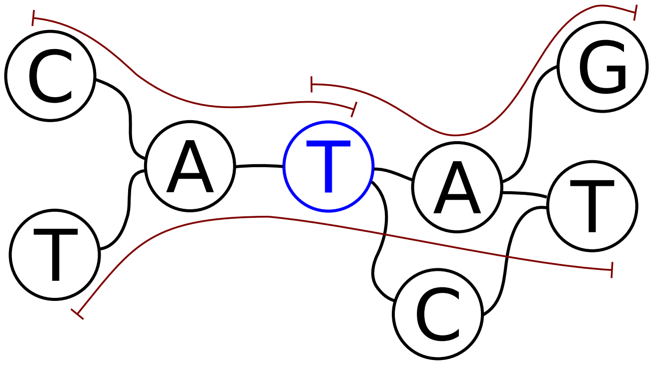


Fig. S6: Generalization of the natural context scheme to graphs. Possible natural contexts (maroon) for a particular "T" base (blue) in a graph are sketched. The contexts are $(\mathtt{CA}, \mathbf{T}, )$, $( , \mathbf{T}, \mathtt{AG})$, and $(\mathtt{TA}, \mathbf{T}, \mathtt{AT})$. These contexts are also minimal, since none can be shortened at either end and still be unique to the "T" in question. A full generalization of the mapping ideas presented here to graph-based reference structures will be presented in a future publication.

in $x$, ordered by ascending start index, in $O(n)$ time. For each MUM instance in the query, ascertaining the maximum number of disjoints MUS instances is linear in the total number of MUS instances it contains. (The problem is an example of the Activity Selection Problem which has a linear, greedy algorithm). The total cost of ascertaining $\alpha'$ for all MUM instances within $x$ is therefore $O(n)$.

A pair $(a, b)$ of distinct MUM instances are **syntenic** if they are in the same relative order and orientation. As one MUM instance on the query can not be contained in another MUM instance, without loss of generality we can assume that the first element of $a$ precedes the first element of $b$, and the last element of $a$ proceeds the last element of $b$. The two MUM instances may partially overlap or be separated by some intervening sequence in the query, and similarly in the reference. Let $c$ and $c'$ be the reference and query substrings of a pair of syntenic MUM instances, such that each substring has the first MUM as a prefix, the second MUM as a suffix and possibly some substring between the two MUMs. The reference substring $c$ may be from the reverse complement of a reference string if the MUM instances are on the reverse strand in the reference. The edit distance between $c$ and $c'$ is the **mismatch gap**; by the definition of a MUM, it must always be one or greater. The mismatch gap can be calculated using the Wagner-Fischer algorithm, which requires time equal to the product of the lengths of $c$ and $c'$. However, this runtime can be improved by noting that the calculated edit distance will be same after first removing the shared prefix of $c$ and $c'$ and then removing the common suffix of the residual strings, the result of which we call the **interstitial substrings** - thus it is easily shown the total cost is bounded by the product of the lengths of the interstitial substrings.

A $\beta'$**-synteny block**, as depicted in Figure 2 in the main text, is a maximal sequence of MUM instances such that each successive pair of elements in the sequence is syntenic and the sum of mismatch gaps between successive pairs is less than or equal to $\beta'$. Let $c$ and $c'$ now be the reference and query substrings of a $\beta'$-synteny block, i.e. the minimal substrings of the reference and query whose prefix

is the first MUM instance in the synteny block and whose suffix is the last MUM instance in the synteny block. Each element in a MUM instance in $c'$ corresponds to an element $i$ in the query and, via the matching, a position $p$ in the reference. For each such $(i, p)$ pair, $c$ is a natural context string for $p$, and $c'$ is a context string with $\beta'$ mismatches from $c$. We call such a context string a **$\beta'$-tolerant context**. Note that $\beta'$ is an upper bound on $\beta$.

The **diagonal** of a MUM instance is equal to the index of its first element in the query string minus the index of its first element in the reference string. Naively, the number of possible pairs of syntenic MUM instances for a query of length $n$ might appear to be $n$ choose 2. However, as we are only interested in $\beta'$-synteny blocks, we do not calculate the mismatch gap between any syntenic pair if the absolute difference between the MUM instance's diagonals is greater than $\beta'$, as such a difference implies an edit distance of greater than $\beta'$. In addition, for a set of MUM instances that have the same diagonal and each form a synteny pair of the form $(a, b)$ with some other MUM instance $b$, we only calculate the mismatch gap between $b$ and the member of this set with greatest final element in the query. This is a heuristic, but in all but the most extreme, contrived cases it works effectively. Finally, we omit calculating the mismatch gap for any synteny pair when either interstitial sequence length is longer than a threshold—here 500bp—and instead set it to positive infinity. Applying these filters and heuristics reduces the total mismatch gap calculation time to $O(\beta' n)$.

The number of $\beta'$-synteny blocks is potentially quite large. However, it is unnecessary to enumerate them. Rather, we need merely to determine if each MUM instance is part of a $\beta'$-synteny block containing $\alpha'$ or more disjoint MUS instances. Given the MUS and MUM instances and the mismatch gap calculations, this step can be achieved in $O(\beta'^2 n)$ time by two passes over the MUS instances. In the first pass, we go through the MUS instances in order of ascending query start position, and, for each MUS instance $b$ and relevant $\beta'$ value ($\leq \beta'$), we calculate $\alpha'$: the maximum number of disjoint MUS instances in a synteny block whose sum of mismatch gaps is at most $\beta'$ and whose final element is $b$. Note that within a MUM, for a given $\beta'$ value, $\alpha'$ for a MUS will be greater than or equal to $\alpha'$ for any MUS starting before it. This can be done by dynamic programming in $O(\beta'^2 n)$ time: each MUS need only look at the latest non-overlapping MUS in each valid predecessor MUM, of which there are $O(\beta)$. In the second pass we repeat the process, but in order of descending query end position, calculating for each MUS instance $b$ and relevant $\beta'$ value ($\leq \beta'$) the maximum number of disjoint MUS instances in a synteny block whose sum of mismatch gaps is at most $\beta'$ and whose first element is $b$. We then combine the information from the two passes, determining for each MUS instance $b$ the maximum number of disjoint MUS instances there can be in a synteny block containing $b$ with at most $\beta'$ mismatches, by scanning through all possible partitions of those mismatches between the left and right sides of the MUS. The maximum of this calculation over all the MUS instances in a MUM instance is then the maximum $\alpha'$ value of a synteny block containing the given MUM instance. We keep only those MUM instances in $\beta'$-tolerant synteny blocks with $\alpha'$ values that equal or exceed $\alpha$.

Using the resulting, filtered subset of MUM instances to map the query elements exactly as in the description for the implementation of the natural context scheme, we derive a heuristic algorithm for the $\alpha$-$\beta$-natural scheme. Our algorithm finds contexts of reference positions in the query string that are at least $\alpha'$-separated, and at most $\beta'$-tolerant, and takes $O(\beta'^2 n)$ time to map the query string, given the previously described substring index structure for the reference. Provided $\alpha' < \beta'$, this context scheme is nonredundant. The contexts found (and thus the matchings made) by this heuristic scheme are a subset of those that would be produced by the exact algorithm, although the same is not always true of the resulting mappings. A more thorough, empirical comparison of this heuristic scheme to an implementation of the exact scheme is left as future work, primarily due to the computational difficulty inherent in nontrivial $\beta$ values.

## REFERENCES


Li, H. (2013). Aligning sequence reads, clone sequences and assembly contigs with bwa-mem. *arXiv preprint arXiv:1303.3997*.

Li, H. and Homer, N. (2010). A survey of sequence alignment algorithms for next-generation sequencing. *Briefings in bioinformatics*, **11**(5), 473–483.

Nguyen, N., Hickey, G., Raney, B. J., Armstrong, J., Clawson, H., Zweig, A., Karolchik, D., Kent, W. J., Haussler, D., and Paten, B. (2014). Comparative assembly hubs: Web-accessible browsers for comparative genomics. *Bioinformatics*, **30**(23), 3293–3301.
